# Supplementary material for: Coda reconstruction from cross-correlation of a diffuse field on thin elastic plates
Source: arXiv:1704.05346 source file (2017-08-25)
Supplement: Supplementary file 1 [file supplementary.pdf]

# Supplemental material on similarity coefficient calculations between a reference cross-correlation and the cross-correlation obtained in two different cases: 1. Time-limited cross-correlation. 2. Instrumental noise affected recordings.


Aida Hejazi Nooghabi,[1,2] Lapo Boschi,[1,3] Philippe Roux,[4] and Julien de Rosny[2]

[1]*Sorbonne Universités, UPMC Univ Paris 06, CNRS, UMR 7193, Institut des Sciences de la Terre de Paris (ISTeP), F-75005 Paris, France*

[2]*ESPCI Paris, PSL Research University, Institut Langevin, 1 rue Jussieu, F-75005, Paris, France*

[3]*Sorbonne Universités, UPMC Univ Paris 06, CNRS, UMR 7190, Institut Jean Le Rond d'Alembert, équipe LAM, F-75005 Paris, France*

[4]*Laboratoire ISTERRE, Université Grenoble Alpes, CNRS, 1380 rue de la Piscine, F-38000, Grenoble, France*



This manuscript contains the calculations of the similarity coefficients for the two cases discussed in the paper entitled 'Coda reconstruction from cross-correlation of a diffuse field on thin elastic plates'. The detailed derivation of the similarity to the best-obtained cross-correlation is provided for two different cases: first, when one signal is cut in time prior to the cross-correlation; and secondly, when the effect of instrumental noise is considered in the cross-correlation. We also compute in details the spatial correlation of the squared eigenmodes for two different geometries which appear in the first two sections. In the last section, we added a table to show the position of the transducers on the plate.


## I. TIME-LIMITED CROSS-CORRELATION AND CONVERGENCE TOWARD THE BEST CROSS-CORRELATION

### A. Relationship between similarity coefficient and variance

We look for the similarity coefficient between the cross-correlation that is obtained by cross-correlation of the two full-time signals averaged over all of the possible point sources ($C_\infty(\mathbf{r}_l^R, \mathbf{r}_{l'}^R, t)$), and the one that is obtained by cross-correlation of a full signal with a windowed one and averaged over a subset of sources ($C_N^{dT}(\mathbf{r}_l^R, \mathbf{r}_{l'}^R, t)$). Here, the subscript and superscript denote the number of sources and the length of the window considered in the cross-correlation, respectively. We write the similarity coefficient between $C_\infty(\mathbf{r}_l^R, \mathbf{r}_{l'}^R, t)$ and $C_N^{dT}(\mathbf{r}_l^R, \mathbf{r}_{l'}^R, t)$ according to the definition of the Pearson correlation coefficient,

$$S(C_\infty, C_N^{dT}) = \frac{\int \left\langle C_N^{dT}(\mathbf{r}_l^R, \mathbf{r}_{l'}^R, t) C_\infty(\mathbf{r}_l^R, \mathbf{r}_{l'}^R, t)\right\rangle dt}{\sqrt{\int \left\langle (C_N^{dT}(\mathbf{r}_l^R, \mathbf{r}_{l'}^R, t))^2\right\rangle dt}\sqrt{\int \left\langle (C_\infty(\mathbf{r}_l^R, \mathbf{r}_{l'}^R, t))^2\right\rangle dt}}. \quad (1.1)$$

We measure $S(C_\infty, C_N^{dT})$. However, on the other hand, as an intermediate step, to analytically estimate $S(C_\infty, C_N^{dT})$, we introduce the fluctuation of $C_N^{dT}$ as

$$C_N^{dT}(\mathbf{r}_l^R, \mathbf{r}_{l'}^R, t) \triangleq \mathscr{C}(\mathbf{r}_l^R, \mathbf{r}_{l'}^R, t) + \delta C_N^{dT}(\mathbf{r}_l^R, \mathbf{r}_{l'}^R, t) \quad (1.2)$$

where $\mathscr{C}(\mathbf{r}_l^R, \mathbf{r}_{l'}^R, t)$ is the cross-correlation obtained by windowing one signal and averaging over a large number of sources and $\delta C_N^{dT}$ is the fluctuation around this value. As both $\mathscr{C}(\mathbf{r}_l^R, \mathbf{r}_{l'}^R, t)$ and $C_\infty(\mathbf{r}_l^R, \mathbf{r}_{l'}^R, t)$ are proportional to the same function $ImG(\mathbf{r}_l^R, \mathbf{r}_{l'}^R, t)$, it is straightforward to show that

$$S(C_\infty, C_N^{dT}) = S(\mathscr{C}, C_N^{dT}) \quad (1.3)$$

Substituting Equation 1.2 into Equation 1.1, the similarity coefficient $S(\mathscr{C}, C_N^{dT})$ can be expressed as:

$$S(\mathscr{C}, C_N^{dT}) = \frac{1}{\sqrt{1 + \frac{\int <\delta C_N^{dT}(\mathbf{r}_l^R, \mathbf{r}_{l'}^R, t)^2> dt}{\int <\mathscr{C}(\mathbf{r}_l^R, \mathbf{r}_{l'}^R, t)^2> dt}}} = \frac{1}{\sqrt{1+Y}} \quad (1.4)$$

where $Y$ is $\frac{\int <\delta C_N^{dT}(\mathbf{r}_l^R, \mathbf{r}_{l'}^R, t)^2> dt}{\int <\mathscr{C}(\mathbf{r}_l^R, \mathbf{r}_{l'}^R, t)^2> dt}$. As a consequence, the estimation of $\mathscr{C}(\mathbf{r}_l^R, \mathbf{r}_{l'}^R, t)$ and $\delta C_N^{dT}(\mathbf{r}_l^R, \mathbf{r}_{l'}^R, t)$ leads to $S(C_\infty, C_N^{dT})$.

### B. Modal expression of the correlation function

The Green's function ($G(\mathbf{r}_l^R, \mathbf{r}_k^S, t)$) expanded in terms of eigen modes ($\phi_n(\mathbf{r})$) and eigen frequencies ($\omega_n$) is written as follows in the frequency domain:

$$G(\mathbf{r}_l^R, \mathbf{r}_k^S, \omega) = \frac{1}{\rho_s} \sum_n \frac{\phi_n(\mathbf{r}_k^S)\phi_n(\mathbf{r}_l^R)}{(\omega^2 - \omega_n^2) - j\frac{\omega}{\alpha_n}}. \tag{1.5}$$

where $\alpha_n$ is the inverse of the decay time of each mode, $\rho_s$ is the surface density, and $\mathbf{r}_k^S$ and $\mathbf{r}_l^R$ are the $k$th source position and the $l$th receiver position, respectively.

This modal representation in the time domain is expressed as

$$G(\mathbf{r}_l^R, \mathbf{r}_k^S, t) = \frac{1}{\rho_s} \sum_n \frac{\phi_n(\mathbf{r}_k^S)\phi_n(\mathbf{r}_l^R)}{\omega_n} exp(-t\alpha_n) sin(\omega_n t). \tag{1.6}$$

What we use as data for the cross-correlation associated to a specific receiver $\mathbf{r}_l^R$ is

$$d(\mathbf{r}_l^R, \mathbf{r}_k^S, t) = G(\mathbf{r}_l^R, \mathbf{r}_k^S, t) \otimes f(t) \tag{1.7}$$

where $f(t)$ is the convolution of the source signal ($f_c(t)$) with its time reversed: $f(t) = f_c(t) \otimes f_c(-t)$. We will have similar data for the second receiver $\mathbf{r}_{l'}^R$, but what we use as the input for computation of the cross-correlation associated to this receiver is this data cut in time, i.e.,

$$d(\mathbf{r}_{l'}^R, \mathbf{r}_k^S, t) = \left[G(r_{l'}^R, \mathbf{r}_k^S, t) \otimes f(t)\right] W(t) \tag{1.8}$$

where $W(t)$ is the window function. The cross-correlation of these two reads as:

$$C(\mathbf{r}_l^R, \mathbf{r}_{l'}^R, t) = \sum_{k=1}^{N} G(r_l^R, \mathbf{r}_k^S, -t) \otimes f(-t) \otimes d(r_{l'}^R, \mathbf{r}_k^S, t) \tag{1.9}$$

where $\otimes$ is the convolution operator.
Substituting $d(\mathbf{r}_{l'}^R, \mathbf{r}_k^S, t)$ gives

$$C(\mathbf{r}_l^R, \mathbf{r}_{l'}^R, t) = \sum_{k=1}^{N} G(\mathbf{r}_l^R, \mathbf{r}_k^S, -t) \otimes f(-t) \otimes \left(\left[G(\mathbf{r}_{l'}^R, \mathbf{r}_k^S, t) \otimes f(t)\right] W(t)\right) \tag{1.10}$$

When the duration of $f(t)$ is much smaller than the length of the window, it is possible to commute $f(t)$ and $W(t)$.

$$C(\mathbf{r}_l^R, \mathbf{r}_{l'}^R, t) \approx \sum_{k=1}^{N} G(\mathbf{r}_l^R, \mathbf{r}_k^S, -t) \otimes f(-t) \otimes \left(G(\mathbf{r}_{l'}^R, \mathbf{r}_k^S, t) W(t)\right) \otimes f(t) \tag{1.11}$$

We denote $f(-t) \otimes f(t)$ as $f'(t)$. Using the definition of convolution

$$C(\mathbf{r}_l^R, \mathbf{r}_{l'}^R, t) \approx \left[\sum_{k=1}^{N} \int G(\mathbf{r}_l^R, \mathbf{r}_k^S, \tau - t) G(\mathbf{r}_{l'}^R, \mathbf{r}_k^S, \tau) W(\tau) d\tau\right] \otimes f'(t) \tag{1.12}$$

From now on, we concentrate on what we have between the brackets, and we represent this as $C_N^{dT}(\mathbf{r}_l^R, \mathbf{r}_{l'}^R, t)$.

$$C_N^{dT}(\mathbf{r}_l^R, \mathbf{r}_{l'}^R, t) = \sum_{k=1}^{N} \int G(\mathbf{r}_l^R, \mathbf{r}_k^S, \tau - t) G(\mathbf{r}_{l'}^R, \mathbf{r}_k^S, \tau) W(\tau) d\tau \tag{1.13}$$

By substituting $G$ from Equation 1.6

$$\begin{aligned} C_N^{dT}(\mathbf{r}_l^R, \mathbf{r}_{l'}^R, t) = \frac{1}{\rho^2} \sum_{k,n,n'} e^{t\alpha_{n'}} \int \frac{\phi_{n'}(\mathbf{r}_k^S)\phi_{n'}(\mathbf{r}_l^R)}{\omega_{n'}} \frac{\phi_n(\mathbf{r}_k^S)\phi_n(\mathbf{r}_{l'}^R)}{\omega_n} \\ \cdot e^{-\tau(\alpha_n + \alpha_{n'})} sin(\omega_n \tau) W(\tau) sin(\omega_{n'}[\tau - t]) H(\tau - t) d\tau \end{aligned} \tag{1.14}$$

Then we use a trigonometry identity. Hence, Equation 1.14 becomes

$$C_N^{dT}(\mathbf{r}_l^R,\mathbf{r}_{l'}^R,t)=\frac{1}{2\rho^2}\sum_{k,n,n'}e^{t\alpha_{n'}}\int\frac{\phi_{n'}(\mathbf{r}_k^S)\phi_{n'}(\mathbf{r}_l^R)}{\omega_{n'}}\frac{\phi_n(\mathbf{r}_k^S)\phi_n(\mathbf{r}_{l'}^R)}{\omega_n}e^{-\tau(\alpha_n+\alpha_{n'})}$$
$$\cdot W(\tau)H(\tau-t)\left[cos(\omega_{n'}t+(\omega_n-\omega_{n'})\tau)-cos((\omega_n+\omega_{n'})\tau-\omega_{n'}t)\right]d\tau \quad (1.15)$$

We now divide this Equation into the separate summations, where $n=n'$ and $n\neq n'$.

$$C_N^{dT}(\mathbf{r}_l^R,\mathbf{r}_{l'}^R,t)=\frac{1}{2\rho^2}e^{t\alpha_n}\int W(\tau)H(\tau-t)e^{-2\tau\alpha_n}d\tau\sum_{k,n}cos(\omega_n t)\frac{\phi_n^2(\mathbf{r}_k^S)\phi_n(\mathbf{r}_l^R)\phi_n(\mathbf{r}_{l'}^R)}{\omega_n^2}$$
$$-\frac{1}{2\rho^2}e^{t\alpha_n}\sum_{k,n}\int W(\tau)H(\tau-t)e^{-2\tau\alpha_n}\frac{\phi_n^2(\mathbf{r}_k^S)\phi_n(\mathbf{r}_l^R)\phi_n(\mathbf{r}_{l'}^R)}{\omega_n^2}cos(2\omega_n\tau-\omega_n t)d\tau$$
$$+\frac{1}{2\rho^2}\sum_{k,n\neq n'}e^{t\alpha_{n'}}\int W(\tau)H(\tau-t)\frac{\phi_{n'}(\mathbf{r}_k^S)\phi_{n'}(\mathbf{r}_l^R)}{\omega_{n'}}\frac{\phi_n(\mathbf{r}_k^S)\phi_n(\mathbf{r}_{l'}^R)}{\omega_n}e^{-\tau(\alpha_n+\alpha_{n'})}$$
$$\cdot\left[cos(\omega_{n'}t+(\omega_n-\omega_{n'})\tau)-cos((\omega_n+\omega_{n'})\tau-\omega_{n'}t)\right]d\tau \quad (1.16)$$

If we assume that the integration time window is long compared to the minimum period, then we can neglect the second term on the right-hand side, and also the term including $cos((\omega_n+\omega_{n'})\tau-\omega_{n'}t)$ in the last term, due to the rapid oscillation with respect to the other terms. We also assume that the attenuation time is not dependent on $n$. So, Equation 1.16 simplifies to

$$C_N^{dT}(\mathbf{r}_l^R,\mathbf{r}_{l'}^R,t)=\frac{1}{2\rho^2}e^{t\alpha_n}\int W(\tau)H(\tau-t)e^{-2\tau\alpha_n}d\tau\sum_{k,n}cos(\omega_n t)\frac{\phi_n^2(\mathbf{r}_k^S)\phi_n(\mathbf{r}_l^R)\phi_n(\mathbf{r}_{l'}^R)}{\omega_n^2}$$
$$+\frac{1}{2\rho^2}\sum_{k,n\neq n'}e^{t\alpha_{n'}}\int\frac{\phi_{n'}(\mathbf{r}_k^S)\phi_{n'}(\mathbf{r}_l^R)}{\omega_{n'}}\frac{\phi_n(\mathbf{r}_k^S)\phi_n(\mathbf{r}_{l'}^R)}{\omega_n}W(\tau)H(\tau-t)e^{-\tau(\alpha_n+\alpha_{n'})}$$
$$\cdot cos(\omega_{n'}t+(\omega_n-\omega_{n'})\tau)d\tau \quad (1.17)$$

Next, we define $\mathscr{C}(\mathbf{r}_l^R,\mathbf{r}_{l'}^R,t)$. This cross-correlation is obtained when there are enough noise sources for $C_N^{dT}(\mathbf{r}_l^R,\mathbf{r}_{l'}^R,t)$; i.e., $\sum_k\phi_n(\mathbf{r}_k^S)\phi_{n'}(\mathbf{r}_k^S)=\delta_{n,n'}N<\phi^2>$[1].

$$\mathscr{C}(\mathbf{r}_l^R,\mathbf{r}_{l'}^R,t)=\frac{N<\phi^2>}{2\rho^2}e^{t\alpha_n}\left(\int W(\tau)H(\tau-t)e^{-2\tau\alpha_n}d\tau\right)\sum_n cos(\omega_n t)\frac{\phi_n(\mathbf{r}_l^R)\phi_n(\mathbf{r}_{l'}^R)}{\omega_n^2} \quad (1.18)$$

## C. Estimation of $\delta C_N^{dT}(\mathbf{r}_l^R,\mathbf{r}_{l'}^R,t)$

We define the variance in $C_N^{dT}(\mathbf{r}_l^R,\mathbf{r}_{l'}^R,t)$ due to the limited number of sources as:

$$\delta C_N^{dT}(\mathbf{r}_l^R,\mathbf{r}_{l'}^R,t)=C_N^{dT}(\mathbf{r}_l^R,\mathbf{r}_{l'}^R,t)-\mathscr{C}(\mathbf{r}_l^R,\mathbf{r}_{l'}^R,t) \quad (1.19)$$

Substituting Equation (1.17) and Equation (1.18) in Equation (1.19)

$$\delta C_N^{dT}(\mathbf{r}_l^R,\mathbf{r}_{l'}^R,t)=$$
$$\frac{1}{2\rho^2}e^{t\alpha_n}\int W(\tau)H(\tau-t)e^{-2\tau\alpha_n}d\tau\sum_{k,n}cos(\omega_n t)\frac{\left(\phi_n^2(\mathbf{r}_k^S)-\langle\phi^2\rangle\right)\phi_n(\mathbf{r}_l^R)\phi_n(\mathbf{r}_{l'}^R)}{\omega_n^2}$$
$$+\frac{1}{2\rho^2}\sum_{k,n\neq n'}e^{t\alpha_{n'}}\int\frac{\phi_{n'}(\mathbf{r}_k^S)\phi_{n'}(\mathbf{r}_l^R)}{\omega_{n'}}\frac{\phi_n(\mathbf{r}_k^S)\phi_n(\mathbf{r}_{l'}^R)}{\omega_n}W(\tau)H(\tau-t)e^{-\tau(\alpha_n+\alpha_{n'})}$$
$$\cdot cos(\omega_{n'}t+(\omega_n-\omega_{n'})\tau)d\tau \quad (1.20)$$

[1] Note that as a consequence of the orthogonality of modes: $\int<\phi^2>dS=1$, $<\phi^2>=1/S$.

We define $\widetilde{M}(\omega_{n'}-\omega_n)$ as the Fourier transform of $W(\tau)H(\tau-t)e^{-\tau(\alpha_n+\alpha_{n'})}$. So, Equation (1.20) reads

$$\begin{aligned}\delta C_N^{dT}(\mathbf{r}_l^R,\mathbf{r}_{l'}^R,t) &= \frac{1}{2\rho^2}e^{t\alpha_n}\widetilde{M}(0)\sum_{k,n} Re e^{j\omega_n t}\frac{\left(\phi_n^2(\mathbf{r}_k^S)-\langle\phi^2\rangle\right)\phi_n(\mathbf{r}_l^R)\phi_n(\mathbf{r}_{l'}^R)}{\omega_n^2}\\ &+\frac{1}{2\rho^2}\sum_{k,n\neq n'} e^{t\alpha_{n'}}\frac{\phi_{n'}(\mathbf{r}_k^S)\phi_{n'}(\mathbf{r}_l^R)}{\omega_{n'}}\frac{\phi_n(\mathbf{r}_k^S)\phi_n(\mathbf{r}_{l'}^R)}{\omega_n}Re[\widetilde{M}(\omega_{n'}-\omega_n)e^{j\omega_{n'}t}]\end{aligned} \tag{1.21}$$

where we assumed that $\alpha_n$ is frequency independent.
Next, we consider the average value of $\delta C_N^{dT}(\mathbf{r}_l^R,\mathbf{r}_{l'}^R,t)^2$.

$$\begin{aligned}\left\langle\delta C_N^{dT}(\mathbf{r}_l^R,\mathbf{r}_{l'}^R,t)^2\right\rangle &= \frac{1}{4\rho^4}e^{2t\alpha_n}\left|\widetilde{M}(0)\right|^2\left[\sum_n\left\langle\left((\sum_k\phi_n^2(\mathbf{r}_k^S))-N\left\langle\phi^2\right\rangle\right)^2\right\rangle\right.\\ &\left.\cdot\frac{<\phi_n^2(\mathbf{r}_l^R)\phi_n^2(\mathbf{r}_{l'}^R)>}{2\omega_n^4}\right]+\frac{1}{8\rho^4}e^{2t\alpha_{n'}}\sum_{n\neq n'}\frac{\left|\widetilde{M}(\omega_{n'}-\omega_n)\right|^2}{\omega_n^2\omega_{n'}^2}\left\langle\left(\sum_k\phi_n(\mathbf{r}_k^S)\phi_{n'}(\mathbf{r}_k^S)\right)\right.\\ &\left.\cdot\left(\sum_{k'}\phi_n(\mathbf{r}_{k'}^S)\phi_{n'}(\mathbf{r}_{k'}^S)\right)\right\rangle\left\langle\phi_n^2(\mathbf{r}_{l'}^R)\right\rangle\left\langle\phi_{n'}^2(\mathbf{r}_l^R)\right\rangle\end{aligned} \tag{1.22}$$

where we neglected the cross term, as the average of the product of the two modes at different locations goes to zero. Let us first look at the first term on the right-hand side of Equation 1.22 and rewrite this as:

$$\begin{aligned}&\frac{1}{4\rho^4}e^{2t\alpha_n}\left|\widetilde{M}(0)\right|^2\left[\sum_n\left\langle\left((\sum_k\phi_n^2(\mathbf{r}_k^S))-N\left\langle\phi^2\right\rangle\right)^2\right\rangle\frac{<\phi_n^2(\mathbf{r}_l^R)\phi_n^2(\mathbf{r}_{l'}^R)>}{2\omega_n^4}\right]=\\ &\frac{1}{4\rho^4}e^{2t\alpha_n}\left|\widetilde{M}(0)\right|^2 N^2<\phi^2>^2\left[\sum_n\left\langle\left((\sum_k\phi_n^2(\mathbf{r}_k^S))/N<\phi^2>-1)\right)^2\right\rangle\right]\\ &\cdot\frac{1}{2}\int\frac{\sum_n\delta(\omega-\omega_n)<\phi_n^2(\mathbf{r}_l^R)\phi_n^2(\mathbf{r}_{l'}^R)>}{\omega^4}d\omega\end{aligned} \tag{1.23}$$

where we used the property of the dirac delta function to replace the sum over $n$ with an integral over a sum of dirac functions.
We next use the definition of modal density ($n_0$) as $n_0(\omega)=\sum_{n=0}^{\infty}\delta(\omega-\omega_n)$. Taking all of this into account, Equation 1.23 reads

$$\begin{aligned}&\frac{1}{4\rho^4}e^{2t\alpha_n}\left|\widetilde{M}(0)\right|^2\left[\sum_n\left\langle\left((\sum_k\phi_n^2(\mathbf{r}_k^S))-N\left\langle\phi^2\right\rangle\right)^2\right\rangle\frac{<\phi_n^2(\mathbf{r}_l^R)\phi_n^2(\mathbf{r}_{l'}^R)>}{2\omega_n^4}\right]=\\ &\frac{1}{4\rho^4}e^{2t\alpha_n}\left|\widetilde{M}(0)\right|^2 N^2<\phi^2>^2\left[\sum_n\left\langle\left((\sum_k\phi_n^2(\mathbf{r}_k^S))/N<\phi^2>-1)\right)^2\right\rangle\right]\\ &\cdot\frac{1}{2}\int\frac{n_0(\omega)}{\omega^4}d\omega[<\phi_n^2(\mathbf{r}_l^R)\phi_n^2(\mathbf{r}_{l'}^R)>]\end{aligned} \tag{1.24}$$

We next evaluate $<\phi_n^2(\mathbf{r}_l^R)\phi_n^2(\mathbf{r}_{l'}^R)>$. Assuming $\phi_n(\mathbf{r}_l^R)$ and $\phi_n(\mathbf{r}_{l'}^R)$ as Gaussian random variables, we can write

$$\begin{aligned}&<\phi_n^2(\mathbf{r}_l^R)\phi_n^2(\mathbf{r}_{l'}^R)>=<\phi_n(\mathbf{r}_l^R)\phi_n(\mathbf{r}_l^R)><\phi_n(\mathbf{r}_{l'}^R)\phi_n(\mathbf{r}_{l'}^R)>\\ &+<\phi_n(\mathbf{r}_l^R)\phi_n(\mathbf{r}_{l'}^R)><\phi_n(\mathbf{r}_l^R)\phi_n(\mathbf{r}_{l'}^R)>\\ &+<\phi_n(\mathbf{r}_l^R)\phi_n(\mathbf{r}_{l'}^R)><\phi_n(\mathbf{r}_l^R)\phi_n(\mathbf{r}_{l'}^R)>=\\ &<\phi^2>^2(1+\frac{2<\phi_n(\mathbf{r}_l^R)\phi_n(\mathbf{r}_{l'}^R)>^2}{<\phi^2>^2})=<\phi^2>^2(1+F(\delta r)).\end{aligned} \tag{1.25}$$

Finally, the first term on the right-hand side of Equation 1.22 becomes

$$\begin{aligned}
&\frac{1}{4\rho^4} e^{2t\alpha_n} \left|\widetilde{M}(0)\right|^2 \left[ \sum_n \left\langle \left( \sum_k \phi_n^2(\mathbf{r}_k^S) - N\left\langle \phi^2 \right\rangle \right)^2 \right\rangle \frac{\left\langle \phi_n^2(\mathbf{r}_l^R)\phi_n^2(\mathbf{r}_{l'}^R) \right\rangle}{2\omega_n^4} \right] = \\
&\frac{1}{8\rho^4} e^{2t\alpha_n} \left|\widetilde{M}(0)\right|^2 \left\langle \phi^2 \right\rangle^4 \left( \int \frac{n_0(\omega)}{\omega^4} d\omega \right) N^2 \left\langle \left( \frac{\sum_k \phi_n^2(\mathbf{r}_k^S)}{N\left\langle \phi^2 \right\rangle} - 1 \right)^2 \right\rangle [1 + F(\delta r)] \\
&= \frac{C_0^2}{\int n_0(\omega) d\omega} \left\langle \left( \frac{\sum_k \phi_n^2(\mathbf{r}_k^S)}{N\left\langle \phi^2 \right\rangle} - 1 \right)^2 \right\rangle [1 + F(\delta r)]
\end{aligned} \tag{1.26}$$

where $C_0^2 = \frac{1}{8\rho^4} e^{2t\alpha_n} \left|\widetilde{M}(0)\right|^2 N^2 < \phi^2 >^4 \frac{1}{\omega^4} (\int n_0(\omega) d\omega)^2$. We assumed that the bandwidth is small enough to take $\frac{1}{\omega^4}$ out of the integral.

We next consider the second term on the right-hand side of Equation 1.22. Let us first simplify $\sum_{n \neq n'} \left|\widetilde{M}(\omega_{n'} - \omega_n)\right|^2$, and write it as

$$\sum_{n \neq n'} \left|\widetilde{M}(\omega_{n'} - \omega_n)\right|^2 = \int_\omega \int_{\omega'} \sum_{n \neq n'} \left|\widetilde{M}(\omega' - \omega)\right|^2 \sum_{n'=0}^{\infty} \delta(\omega' - \omega_{n'}) \sum_{n=0}^{\infty} \delta(\omega - \omega_n) d\omega' d\omega \tag{1.27}$$

We see that the definition of modal density appears. We now define $\kappa(\delta\omega, \omega) = \frac{< n_0(\omega) n_0(\omega + \delta\omega) >}{n_0(\omega)}$

$$\sum_{n \neq n'} \left|\widetilde{M}(\omega_{n'} - \omega_n)\right|^2 = \int \int n_0(\omega) \kappa(\delta\omega, \omega)) \left|\widetilde{M}(\delta\omega)\right|^2 d\delta\omega d\omega \tag{1.28}$$

And hence the second term on the right-hand side of Equation 1.22 reads

$$\begin{aligned}
&\frac{1}{8\rho^4} e^{2t\alpha_{n'}} \sum_{n \neq n'} \frac{\left|\widetilde{M}(\omega_{n'} - \omega_n)\right|^2}{\omega_n^2 \omega_{n'}^2} \left\langle \left( \sum_k \phi_n(\mathbf{r}_k^S) \phi_{n'}(\mathbf{r}_k^S) \right) \left( \sum_{k'} \phi_n(\mathbf{r}_{k'}^S) \phi_{n'}(\mathbf{r}_{k'}^S) \right) \right\rangle \\
&\cdot \left\langle \phi_n^2(\mathbf{r}_l^R) \right\rangle \left\langle \phi_{n'}^2(\mathbf{r}_{l'}^R) \right\rangle = \frac{1}{8\rho^4} e^{2t\alpha_{n'}} \left|\widetilde{M}(0)\right|^2 N^2 \int \frac{n_0(\omega)}{\omega^4} d\omega \left\langle \phi^2 \right\rangle^4 \\
&\cdot \left( \int \kappa(\delta\omega, \omega) \frac{\left|\widetilde{M}(\delta\omega)\right|^2}{\left|\widetilde{M}(0)\right|^2} d\delta\omega \right) \frac{\left\langle \left( \sum_k \phi_n(\mathbf{r}_k^S) \phi_{n'}(\mathbf{r}_k^S) \right)^2 \right\rangle}{N^2 \left\langle \phi^2 \right\rangle^2} = \\
&\frac{C_0^2}{\int n_0(\omega) d\omega} \left( \int \kappa(\delta\omega, \omega) \frac{\left|\widetilde{M}(\delta\omega)\right|^2}{\left|\widetilde{M}(0)\right|^2} d\delta\omega \right) \frac{\left\langle \left( \sum_k \phi_n(\mathbf{r}_k^S) \phi_{n'}(\mathbf{r}_k^S) \right)^2 \right\rangle}{N^2 \left\langle \phi^2 \right\rangle^2}
\end{aligned} \tag{1.29}$$

So, finally, Equation 1.22 becomes

$$\begin{aligned}
&\left\langle \delta C_N^{dT}(\mathbf{r}_l^R, \mathbf{r}_{l'}^R, t)^2 \right\rangle = \frac{C_0^2}{\int n_0(\omega) d\omega} \left[ \left\langle \left( \sum \phi_n^2(\mathbf{r}_k^S)/N\left\langle \phi^2 \right\rangle - 1 \right)^2 \right\rangle \right. \\
&\cdot [1 + F(\delta r)] + \left( \int \kappa(\delta\omega, \omega) \frac{\left|\widetilde{M}(\delta\omega)\right|^2}{\left|\widetilde{M}(0)\right|^2} d\ \delta\omega \right) \\
&\left. \cdot \frac{\left\langle \left( \sum_k \phi_n(\mathbf{r}_k^S) \phi_{n'}(\mathbf{r}_k^S) \right)^2 \right\rangle}{N^2 \left\langle \phi^2 \right\rangle^2} \right]
\end{aligned} \tag{1.30}$$

### D. Estimation of $\langle \mathscr{C}(\mathbf{r}_l^R, \mathbf{r}_{l'}^R, t)^2 \rangle$

From Equation (1.18),

$$\begin{aligned} \langle \mathscr{C}(\mathbf{r}_l^R, \mathbf{r}_{l'}^R, t)^2 \rangle = & \frac{N^2 <\phi^2>^2}{4\rho^4} e^{2t\alpha_n} \left( \int W(\tau) H(\tau - t) e^{-2\tau\alpha_n} d\tau \right)^2 \\ & \left( \sum_n cos^2(\omega_n t) \frac{\langle \phi_n^2(\mathbf{r}_l^R) \phi_n^2(\mathbf{r}_{l'}^R) \rangle}{\omega_n^4} + \sum_{n \neq n'} cos(\omega_n t) cos(\omega_{n'} t) \frac{\langle \phi_n(\mathbf{r}_l^R) \phi_{n'}(\mathbf{r}_{l'}^R) \rangle^2}{\omega_n^2 \omega_{n'}^2} \right). \end{aligned} \tag{1.31}$$

Taking the integral and neglecting the rapidly oscillating terms,

$$\begin{aligned} \left\langle \int \mathscr{C}(\mathbf{r}_l^R, \mathbf{r}_{l'}^R, t)^2 dt \right\rangle = & \frac{N^2 <\phi^2>^2}{4\rho^4} \int (e^{2t\alpha_n} \left( \int W(\tau) H(\tau - t) e^{-2\tau\alpha_n} d\tau \right)^2 \\ & \sum_n \frac{\langle \phi_n^2(\mathbf{r}_l^R) \phi_n^2(\mathbf{r}_{l'}^R) \rangle}{2\omega_n^4} + \sum_{n \neq n'} cos((\omega_n - \omega_{n'})\, t) \frac{\langle \phi_n(\mathbf{r}_l^R) \phi_{n'}(\mathbf{r}_{l'}^R) \rangle^2}{2\omega_n^4} ) dt \end{aligned} \tag{1.32}$$

As for the previous section, the introduction of the modal density and the modal density correlation function leads to

$$\begin{aligned} \left\langle \int \mathscr{C}(\mathbf{r}_l^R, \mathbf{r}_{l'}^R, t)^2 dt \right\rangle = & \frac{N^2 <\phi^2>^2}{8\rho^4} \int \frac{n_0(\omega) d\omega}{\omega^4} \int (e^{2t\alpha_n} \left( \int W(\tau) H(\tau - t) e^{-2\tau\alpha_n} d\tau \right)^2 \\ & \left( \langle \phi_n^2(\mathbf{r}_l^R) \phi_n^2(\mathbf{r}_{l'}^R) \rangle + \kappa(t) \langle \phi_n(\mathbf{r}_l^R) \phi_n(\mathbf{r}_{l'}^R) \rangle^2 \right) ) dt \end{aligned} \tag{1.33}$$

where $\kappa(t)$ is the inverse Fourier transform of $\kappa(\delta\omega)$. As $\kappa(\delta\omega) = n_0$ for a regular cavity, $\kappa(t) = n_0 \delta(t)$. The second term can thus be neglected because it is only significant when t=0 and $\mathbf{r}_l^R = \mathbf{r}_{l'}^R$. Then,

$$\left\langle \int \mathscr{C}(\mathbf{r}_l^R, \mathbf{r}_{l'}^R, t)^2 dt \right\rangle \approx \frac{(1 + F(\delta r))}{\int n_0(\omega) d\omega} \int C_0^2 dt. \tag{1.34}$$

### E. Estimation of the similarity coefficient $S(C_\infty, C_N^{dT})$

Substituting Equation 1.30 and Equation 1.34, $Y$ reads

$$\begin{aligned} Y = & \left\langle \left( \sum_k \phi_n^2(\mathbf{r}_k^S) / N \langle \phi^2 \rangle - 1 \right)^2 \right\rangle \\ & + \frac{\left( \int \kappa(\delta\omega, \omega) \frac{|\widetilde{M}(\delta\omega)|^2}{|\widetilde{M}(0)|^2} d\delta\omega \right) \frac{\left\langle \left( \sum_k \phi_n(\mathbf{r}_k^S) \phi_{n'}(\mathbf{r}_k^S) \right)^2 \right\rangle}{N^2 \langle \phi^2 \rangle^2}}{1 + F(\delta r)} \end{aligned} \tag{1.35}$$

Before going further, we simplify this Equation.
First, we consider $\left\langle \left( \sum_k \phi_n^2(\mathbf{r}_k^S) / N \langle \phi^2 \rangle - 1 \right)^2 \right\rangle$ and rewrite it as $\left\langle \left( \frac{1}{N} \sum_k a_k^2 - 1 \right)^2 \right\rangle$, where $a_k^2 = \frac{\phi_n^2(\mathbf{r}_k^S)}{\langle \phi^2 \rangle}$.

$$\begin{aligned} & \left\langle \left( \frac{1}{N} \sum_k a_k^2 - 1 \right)^2 \right\rangle = \frac{1}{N^2} \sum_{k,k'=1}^{N} \langle a_k^2 a_{k'}^2 \rangle + 1 - \frac{2}{N} \left\langle \sum_{k=1}^{N} a_k^2 \right\rangle = \\ & \frac{1}{N^2} \left[ 3N \langle a_k^2 \rangle^2 + N(N-1) \langle a_k^2 \rangle^2 \right] - 1 = \frac{2}{N} \langle a_k^2 \rangle^2 + \langle a_k^2 \rangle^2 - 1 = \frac{2}{N} \end{aligned} \tag{1.36}$$

Next, we consider $\left\langle \left(\sum_k \phi_n(\mathbf{r}_k^S)\phi_{n'}(\mathbf{r}_k^S)\right)^2\right\rangle$.

$$\begin{gathered}\left\langle \left(\sum_k \phi_n(\mathbf{r}_k^S)\phi_{n'}(\mathbf{r}_k^S)\right)^2\right\rangle = \sum_{k,k'=1}^{N} \left\langle \phi_n(\mathbf{r}_k^S)\phi_n(\mathbf{r}_{k'}^S)\phi_{n'}(\mathbf{r}_k^S)\phi_{n'}(\mathbf{r}_{k'}^S)\right\rangle = \\ \sum_{k,k'=1}^{N} \left\langle \phi_n(\mathbf{r}_k^S)\phi_n(\mathbf{r}_{k'}^S)\right\rangle \left\langle \phi_{n'}(\mathbf{r}_k^S)\phi_{n'}(\mathbf{r}_{k'}^S)\right\rangle = N\left\langle \phi^2\right\rangle^2\end{gathered} \tag{1.37}$$

Using Equation 1.36 and Equation 1.37, $Y$ simplifies to

$$Y = \frac{\frac{2}{N}\left[1+F(\delta r)\right] + \left(\int \kappa(\delta\omega,\omega))\frac{\left|\widetilde{M}(\delta\omega)\right|^2}{\left|\widetilde{M}(0)\right|^2} d\delta\omega\right)\frac{1}{N}}{1+F(\delta r)} \tag{1.38}$$

Substituting Equation 1.38 in Equation 1.4, the similarity coefficient $S(C_\infty, C_N^{dT})$ reads

$$S(C_\infty, C_N^{dT}) = \frac{1}{\sqrt{1+\frac{\frac{2}{N}[1+F(\delta r)]+\left(\int \kappa(\delta\omega,\omega))\frac{\left|\widetilde{M}(\delta\omega)\right|^2}{\left|\widetilde{M}(0)\right|^2}d\delta\omega\right)\frac{1}{N}}{1+F(\delta r)}}} \tag{1.39}$$

We assume that $\kappa(\delta\omega,\omega)$ is equal to the average value of the modal density. We next simplify $\int \frac{\left|\widetilde{M}(\delta\omega)\right|^2}{\left|\widetilde{M}(0)\right|^2} d\delta\omega$. If we replace $\omega' - \omega = \omega$ and $\alpha_n = \alpha_{n'}$, then according to the definition of the Fourier transform

$$\widetilde{M}(\omega) = \int_{T_{min}}^{T_{max}} e^{-2\alpha\tau} e^{-j\omega\tau} d\tau = \frac{e^{-i\omega T_{min} - 2\alpha T_{min}}}{i\omega + 2\alpha} - \frac{e^{-i\omega T_{max} - 2\alpha T_{max}}}{i\omega + 2\alpha}, \tag{1.40}$$

and

$$\widetilde{M}(0) = \int_{T_{min}}^{T_{max}} e^{-2\alpha\tau} d\tau = \frac{e^{-2\alpha T_{min}}}{2\alpha} - \frac{e^{-2\alpha T_{max}}}{2\alpha}. \tag{1.41}$$

Using Equation (1.40) and Equation (1.41),

$$\int \frac{\left|\widetilde{M}(\omega)\right|^2}{\left|\widetilde{M}(0)\right|^2} d\omega = \frac{2\pi\alpha(e^{2\alpha T_{max}} + e^{2\alpha T_{min}})}{(e^{\alpha T_{max}} - e^{\alpha T_{min}})(e^{\alpha T_{max}} + e^{\alpha T_{min}})} = 2\pi\alpha coth(\alpha(T_{max} - T_{min})). \tag{1.42}$$

And finally $S(C_\infty, C_N^{dT})$ reads

$$S(C_\infty, C_N^{dT}) = \frac{1}{\sqrt{1+\frac{\frac{2}{N}[1+F(\delta r)]+(n_0(\omega)2\pi\alpha coth(\alpha(T_{max}-T_{min})))\frac{1}{N}}{1+F(\delta r)}}}. \tag{1.43}$$

## II. INSTRUMENTAL-NOISE AFFECTED RECORDINGS AND CONVERGENCE TOWARD THE BEST CROSS-CORRELATION

In this part, we quantify the contribution of the noise. In other words, we only consider the effects of variations in the cross-correlation induced by noise and not by the insufficient number of sources (the latter case is studied in part I in detail). To this end, we cross-correlate two time-windowed signals in the coda part of the recordings. The reason why we do not cross-correlate a windowed signal with the full-time signal is that in this case the effects of the noise will not be finite. Here, we look for the similarity coefficient between the cross-correlation obtained between the two windowed signals considering all of the available sources ($C_\infty^{dT}$) and the reference source ($C_\infty$). We write the similarity coefficient $S(C_\infty, C_\infty^{dT})$ as:

$$S(C_\infty, C_\infty^{dT}) = \frac{\int \left\langle C_\infty^{dT}(\mathbf{r}_l^R, \mathbf{r}_{l'}^R, t) C_\infty(\mathbf{r}_l^R, \mathbf{r}_{l'}^R, t)\right\rangle dt}{\sqrt{\int \left\langle (C_\infty^{dT}(\mathbf{r}_l^R, \mathbf{r}_{l'}^R, t))^2\right\rangle dt}\sqrt{\int \left\langle (C_\infty(\mathbf{r}_l^R, \mathbf{r}_{l'}^R, t))^2\right\rangle dt}} \tag{2.1}$$

Similar to the previous section, we introduce the fluctuation of $C_{\infty}^{dT}$ as:

$$C_{\infty}^{dT}(\mathbf{r}_l^R, \mathbf{r}_{l'}^R, t) \triangleq \mathscr{C}'(\mathbf{r}_l^R, \mathbf{r}_{l'}^R, t) + \delta n(t) \tag{2.2}$$

where $\delta n(t)$ is the variance in the obtained cross-correlation due to the instrumental noise, and $\mathscr{C}'(\mathbf{r}_l^R, \mathbf{r}_{l'}^R, t)$ is the ideal cross-correlation obtained by cross-correlation of two time-limited windows when there are sufficient noise sources.

Substituting Equation 2.2 into Equation 2.1, the simplified $S(C_\infty, C_\infty^{dT})$ is written as:

$$S(C_\infty, C_\infty^{dT}) = \frac{1}{\sqrt{1 + \frac{\int <\delta n(\mathbf{r}_l^R, \mathbf{r}_{l'}^R, t)^2> dt}{\int <C_\infty(\mathbf{r}_l^R, \mathbf{r}_{l'}^R, t)^2> dt}}} = \frac{1}{\sqrt{1+Z}} \tag{2.3}$$

where $Z$ is $\frac{\int <\delta n(\mathbf{r}_l^R, \mathbf{r}_{l'}^R, t)^2> dt}{\int <C_\infty(\mathbf{r}_l^R, \mathbf{r}_{l'}^R, t)^2> dt}$. Similar to the previous section, and because $\mathscr{C}'(\mathbf{r}_l^R, \mathbf{r}_{l'}^R, t)$ and $C_\infty(\mathbf{r}_l^R, \mathbf{r}_{l'}^R, t)$ are proportional to $ImG(\mathbf{r}_l^R, \mathbf{r}_{l'}^R, t)$,

$$S(C_\infty, C_\infty^{dT}) = S(\mathscr{C}', C_\infty^{dT}) \tag{2.4}$$

and hence $Z$ can be rewritten as $\frac{\int <\delta n(\mathbf{r}_l^R, \mathbf{r}_{l'}^R, t)^2> dt}{\int <\mathscr{C}'(\mathbf{r}_l^R, \mathbf{r}_{l'}^R, t)^2> dt}$.

The goal here is to consider the effects of electronic noise on the cross-correlations, and hence on the similarity coefficient.

We assume that the estimated Green's function ($G_m(\mathbf{r}_l^R, \mathbf{r}_k^S, t)$) coincides with the sum of the exact Green's function $G(\mathbf{r}_l^R, \mathbf{r}_k^S, t)$, and the instrument-related error $n$

$$G_m(\mathbf{r}_l^R, \mathbf{r}_k^S, t) = G(\mathbf{r}_l^R, \mathbf{r}_k^S, t) + n(t) \tag{2.5}$$

In the experimental case, we cross-correlate the two windowed recordings and call this $C_\infty^{dT}(\mathbf{r}_l^R, \mathbf{r}_k^S, t)$. Here, we temporarily, and from a theoretical point of view, call $C_\infty^{dT}(\mathbf{r}_l^R, \mathbf{r}_k^S, t)$ as $C_{N,n}^{dT}(\mathbf{r}_l^R, \mathbf{r}_k^S, t)$ to emphasize that the cross-correlations are affected by the noise ($n$). Applying the definition of cross-correlation, $C_{N,n}^{dT}(\mathbf{r}_l^R, \mathbf{r}_k^S, t)$ reads

$$C_{N,n}^{dT}(\mathbf{r}_l^R, \mathbf{r}_{l'}^R, t) = \sum_k \int \left[G(\mathbf{r}_k^S, \mathbf{r}_l^R, \tau - t) + n_{l,k}(\tau - t)\right] W(\tau - t) \left[G(\mathbf{r}_k^S, \mathbf{r}_{l'}^R, \tau) + n_{l',k}(\tau)\right] W(\tau) d\tau \tag{2.6}$$

The cross-correlations are summed over all of the available sources located at $r_k^S$.

To get $Z$, we first calculate

$$\begin{aligned}\left\langle C_{N,n}^{dT}(\mathbf{r}_l^R, \mathbf{r}_{l'}^R, t)^2\right\rangle = \left\langle \mathscr{C}_0'^2(\mathbf{r}_l^R, \mathbf{r}_{l'}^R, t)\right\rangle + \int \left\langle G^2(\mathbf{r}_k^S, \mathbf{r}_l^R, \tau - t)\right\rangle H(\tau - t) W(\tau) d\tau \int n_{l',k}^2(\tau) W(\tau') d\tau' + \\ \int \left\langle G^2(\mathbf{r}_k^S, \mathbf{r}_l^R, \tau)\right\rangle W(\tau) d\tau \int n_{l',k}^2(\tau') W(\tau' - t) d\tau' + \left(\int n_{l',k}^2 W(\tau' - t) d\tau'\right)^2\end{aligned} \tag{2.7}$$

where $\mathscr{C}_0'(\mathbf{r}_l^R, \mathbf{r}_{l'}^R, t)$ is the product of the $G$s that are not disturbed by the noise (indicated by subscript 0).

We first compute $\left\langle G^2(\mathbf{r}_k^S, \mathbf{r}_l^R, \tau)\right\rangle$. Using the modal expansion of the Green's function,

$$G(\mathbf{r}_k^S, \mathbf{r}_l^R, t) = \frac{1}{\rho_s} \sum_n \frac{\phi_n(\mathbf{r}_k^S)\phi_n(\mathbf{r}_l^R)}{\omega_n} exp(-t\alpha_n) sin(\omega_n t). \tag{2.8}$$

$G^2(\mathbf{r}_k^S, \mathbf{r}_l^R, \tau)$ reads

$$G^2(\mathbf{r}_k^S, \mathbf{r}_l^R, \tau) = \frac{1}{2\rho_s^2} \sum_{n,n'} \frac{\phi_n(\mathbf{r}_k^S)\phi_n(\mathbf{r}_l^R)\phi_{n'}(\mathbf{r}_k^S)\phi_{n'}(\mathbf{r}_l^R)}{\omega_n \omega_{n'}} exp(-t(\alpha_n + \alpha_{n'})) \left[cos(\omega_n - \omega_{n'})t - cos(\omega_n + \omega_{n'})t\right] \tag{2.9}$$

where we used the trigonometry identity.

Neglecting the rapidly oscillating terms and rewriting $G^2(\mathbf{r}_k^S, \mathbf{r}_l^R, \tau)$ as the sum of two terms for $n \neq n'$ and $n = n'$, gives

$$G^2(\mathbf{r}_k^S, \mathbf{r}_l^R, \tau) = \frac{1}{2\rho_s^2} \sum_{n \neq n'} \frac{exp(-t(\alpha_n + \alpha_{n'}))\phi_n(\mathbf{r}_k^S)\phi_n(\mathbf{r}_l^R)\phi_{n'}(\mathbf{r}_k^S)\phi_{n'}(\mathbf{r}_l^R)}{\omega_n \omega_{n'}}(cos(\omega_n - \omega_{n'})t) + \frac{1}{2\rho_s^2} \sum_n \frac{exp(-2t\alpha_n)\phi_n^2(\mathbf{r}_k^S)\phi_n^2(\mathbf{r}_l^R)}{\omega_n^2} \tag{2.10}$$

Using Equation 1.25 and considering $< \phi_n(\mathbf{r}_k^S)\phi_n(\mathbf{r}_l^R) >= 0$, $\langle G^2(\mathbf{r}_k^S, \mathbf{r}_l^R, \tau)\rangle$ becomes

$$\langle G^2(\mathbf{r}_k^S, \mathbf{r}_l^R, \tau)\rangle = \frac{e^{-2\tau\alpha_n}}{2{\rho_s}^2} \sum \frac{\langle\phi^2\rangle^2 (1 + F(\delta r))}{\omega_n^2} = \frac{\langle\phi^2\rangle^2 e^{-2\tau\alpha_n}(1 + F(\delta r))}{2\rho_s^2} \int \frac{n_0(\omega)}{\omega^2} d\omega \tag{2.11}$$

and subsequently

$$\int \langle G^2(\mathbf{r}_k^S, \mathbf{r}_l^R, \tau - t)\rangle H(\tau - t)W(\tau)d\tau = \frac{\langle\phi^2\rangle^2 (1 + F(\delta r)) \int e^{-2(\tau - t)\alpha_n} H(\tau - t)W(\tau)d\tau}{2{\rho_s}^2} \int \frac{n_0(\omega)}{\omega^2} d\omega \tag{2.12}$$

Assuming $n$ to be white noise, $n^2$ is equal to $\Pi_n B$, where $\Pi_n$ and $B$ are the noise level and the bandwidth, respectively. Hence, Equation 2.7 becomes

$$\langle C_{N,n}^{dT}(\mathbf{r}_l^R, \mathbf{r}_{l'}^R, t)^2\rangle = \left\langle \mathscr{C}_0'(\mathbf{r}_l^R, \mathbf{r}_{l'}^R, t)^2 \right\rangle + \frac{\mathscr{C}'(\mathbf{r}_l^R, \mathbf{r}_{l'}^R, t = 0)\left[1 + F(\delta r)\right]}{N} \left[\frac{\int e^{-2(t-\tau)\alpha_n} H(\tau - t)W(\tau)d\tau}{\int e^{-2\tau\alpha_n} W(\tau)d\tau} + 1\right] \Pi_n B[T_{max} - T_{min}] + \left(\Pi_n B[T_{max} - T_{min}]\right)^2 \tag{2.13}$$

$\mathscr{C}'(\mathbf{r}_l^R, \mathbf{r}_{l'}^R, t)$ is obtained by cross-correlation of two time-limited windows when there are enough noise sources. On the other hand, using Equation 1.18, we can write $\mathscr{C}'(\mathbf{r}_l^R, \mathbf{r}_{l'}^R, t)$ as

$$\mathscr{C}'(\mathbf{r}_l^R, \mathbf{r}_{l'}^R, t) = \frac{N < \phi^2 >}{2\rho_s^2} e^{t\alpha_n} \left(\int W(\tau)W(\tau - t)e^{-2\tau\alpha} d\tau\right) \sum_n cos(\omega_n t) \frac{\phi_n(\mathbf{r}_l^R)\phi_n(\mathbf{r}_{l'}^R)}{\omega_n^2} \tag{2.14}$$

So,

$$\mathscr{C}'(\mathbf{r}_l^R, \mathbf{r}_{l'}^R, t = 0) = \frac{N < \phi^2 >}{2\rho_s^2} \left(\int_{T_{min}}^{T_{max}} W(\tau)e^{-2\tau\alpha} d\tau\right) \int \frac{n_0(\omega)}{\omega^2} d\omega \tag{2.15}$$

and

$$\mathscr{C}'(\mathbf{r}_l^R, \mathbf{r}_{l'}^R, t = 0) = \frac{N < \phi^2 >}{4\alpha\rho_s^2} (\int \frac{n_0(\omega)}{\omega^2} d\omega)(e^{-2\alpha T_{min}} - e^{-2\alpha T_{max}}) \tag{2.16}$$

And we can write

$$< (\mathscr{C}'(\mathbf{r}_l^R, \mathbf{r}_{l'}^R, t))^2 >= \mathscr{C}'(\mathbf{r}_l^R, \mathbf{r}_{l'}^R, t = 0)^2 \left[\frac{e^{-2\alpha T_{min}} - e^{-2\alpha(T_{max} - t)}}{e^{-2\alpha T_{min}} - e^{-2\alpha T_{max}}}\right]^2 \frac{(1 + F(\delta r))}{2\int n_0(\omega)d\omega} \tag{2.17}$$

and the variations in the cross-correlation due to the noise are

$$\left\langle C_{N,n}^{dT}(\mathbf{r}_l^R,\mathbf{r}_{l'}^R,t)^2\right\rangle - \left\langle \mathscr{C}'(\mathbf{r}_l^R,\mathbf{r}_{l'}^R,t)^2\right\rangle = \tag{2.18}$$

$$\frac{\mathscr{C}'(\mathbf{r}_l^R,\mathbf{r}_{l'}^R,t=0)\,[1+F(\delta r)]}{N}\left[\frac{\int e^{-2(t-\tau)\alpha_n}H(\tau-t)W(\tau)d\tau}{\int e^{-2\tau\alpha_n}W(\tau)d\tau}+1\right]\Pi_n B[T_{max}-T_{min}] \tag{2.19}$$

$$+\left(\Pi_n B[T_{max}-T_{min}]\right)^2$$

Substituting for $Z$, gives,

$$1+Z = 1+\frac{\int \mathscr{C}'(\mathbf{r}_l^R,\mathbf{r}_{l'}^R,t=0)\,[1+F(\delta r)]\,dt}{N\int <(\mathscr{C}'(\mathbf{r}_l^R,\mathbf{r}_{l'}^R,t))^2>dt}\left[\int\left(\frac{\int e^{-2(t-\tau)\alpha_n}H(\tau-t)W(\tau)d\tau}{\int e^{-2\tau\alpha_n}W(\tau)d\tau}+1\right)dt\right]\Pi_n B[T_{max}-T_{min}]$$
$$+\frac{\int\left(\Pi_n B[T_{max}-T_{min}]\right)^2 dt}{\int <(\mathscr{C}'(\mathbf{r}_l^R,\mathbf{r}_{l'}^R,t))^2>dt} \tag{2.20}$$

or,

$$1+Z = 1+\frac{\int n_0(\omega)d\omega}{N\mathscr{C}'(\mathbf{r}_l^R,\mathbf{r}_{l'}^R,t=0)}\left[\frac{\int\left(\frac{\int e^{-2(t-\tau)\alpha_n}H(\tau-t)W(\tau)d\tau}{\int e^{-2\tau\alpha_n}W(\tau)d\tau}+1\right)dt}{\int\left[\frac{e^{-2\alpha T_{min}}-e^{-2\alpha(T_{max}-t)}}{e^{-2\alpha T_{min}}-e^{-2\alpha T_{max}}}\right]^2 dt}\right]\frac{\Pi_n B[T_{max}-T_{min}]}{\alpha_n\int W(\tau)e^{-2\tau\alpha_n}d\tau(1+F(\delta r))}$$
$$+\frac{\int\left(\Pi_n B[T_{max}-T_{min}]\right)^2 dt}{\int <(\mathscr{C}'(\mathbf{r}_l^R,\mathbf{r}_{l'}^R,t))^2>dt} \tag{2.21}$$

We next apply a simplification and neglect the last term, as it is of the second order.

Assuming a small t ($t\approx 0$), the term in the brackets simplifies to 2, and the similarity coefficient can be finally expressed as:

$$S(C_\infty,C_\infty^{dT}) \approx \left(1+\frac{\beta B[T_{max}-T_{min}]}{N(e^{-T_{min}/\tau_a}-e^{-T_{max}/\tau_a})}\right)^{-0.5} \tag{2.22}$$

where

$$\beta = \frac{2\Pi_n}{\mathscr{C}'(\mathbf{r}_l^R,\mathbf{r}_{l'}^R,t=0)(1+F(\delta r))}. \tag{2.23}$$

The dimensionless value $\beta$ indicates the noise-to-signal ratio.

## III. SPATIAL CORRELATION OF THE SQUARED EIGEN-MODES

In the last section of this material, we derive the expression for the spatial correlation of the squared eigen modes $<\phi_n^2(\mathbf{r})\phi_n^2(\mathbf{r}')>$ and the expression of F (that appeared in the calculus of the similarity coefficient in both previous sections) for two different cases: Chaotic geometry and integrable cavity. Here, $\mathbf{r}$ and $\mathbf{r}'$ can be considered as the generalized form for $(\mathbf{r}_l^R)$ and $(\mathbf{r}_{l'}^R)$.

- **Chaotic geometry**

In case of a chaotic geometry, Berry stated that the eigenmodes behave as Gaussian variables with a spatial correlation given by

$$\langle\phi_n(\mathbf{r})\phi_n(\mathbf{r}')\rangle = \langle\phi\rangle^2 J_0(k\delta r). \tag{3.1}$$

The relationship between the fourth order moment of a Gaussian variable in terms of second order moments (similar to Eq. (1.25)) yields

$$\left\langle \phi_n^2(\mathbf{r})\phi_n^2(\mathbf{r}')\right\rangle = \left\langle \phi_n^2(\mathbf{r})\right\rangle \left\langle \phi_n^2(\mathbf{r}')\right\rangle + 2\left\langle \phi_n(\mathbf{r})\phi_n(\mathbf{r}')\right\rangle^2 . \tag{3.2}$$

Using Eq. (3.1), it comes

$$\left\langle \phi_n^2(\mathbf{r})\phi_n^2(\mathbf{r}')\right\rangle = \left\langle \phi^2\right\rangle^2 \left[1 + 2J_0(k\delta r)^2\right], \tag{3.3}$$

and therefore

$$F(\delta r) = 2J_0(k\delta r)^2 \tag{3.4}$$

- **Integrable cavity**

For a clamped rectangular plate, the expression of the eigenmode separated in two dimensions ($x$ and $y$) is given by

$$\phi(x, y) = \frac{2\sin(k_x x)\sin(k_y y)}{\sqrt{A}}, \tag{3.5}$$

where $A$ is the plate area (e.g.[1]). For simplicity in this section, we drop $n$ (which normally appears as the subscript for $\phi$ and the coefficient for $k$ in the argument of $sin$).

We compute $\left\langle \phi^2(x, y)\phi^2(x', y')\right\rangle$ in a similar manner to the one used in [1] to estimate the spatial correlation of the eigenmodes. Strictly speaking, the averaging has to be performed by integrating over a quarter of a ring of radius $k$ and thickness $dk$ (positive $k_x$ and $k_y$). However here, to facilitate the calculus and without amending the result, the integration is done over the full ring,

$$\left\langle \phi^2(x, y)\phi^2(x', y')\right\rangle = \frac{16}{A^2 2\pi k\delta k}\int_0^{2\pi}\int_k^{k+\delta k} \left\langle \sin^2(k_x x)\sin^2(k_y y)\sin^2(k_x x')\sin^2(k_y y')\right\rangle kdkd\theta, \tag{3.6}$$

with $k_x = kcos\theta$ and $k_y = ksin\theta$.

This integral can be estimated using the following trigonometric identity

$$sin^2(k_x x)sin^2(k_x x') = \frac{(1 - \cos(2k_x x) - \cos(2k_x x'))}{4} + \frac{\cos(2k_x[x - x']) + \cos(2k_x[x + x'])}{8}. \tag{3.7}$$

Similar to [1], an expression that is valid for all $x$ and $x'$ can be worked out. However, for the sake of simplicity, we assume here that the position coordinates $x$ and $x'$ are sufficiently far (farther than a couple of wavelengths) from the plate borders. In such a case, only the terms $1/4$ and $cos(2k_x[x - x'])$ significantly contribute to the integral because the other terms oscillate much faster with respect to $k_x$. The same goes for $k_y$ terms in Eq. (3.6).

Finally, it comes

$$\left\langle \phi^2(x, y)\phi^2(x', y')\right\rangle = \frac{1}{A^2 2\pi}\int_0^{2\pi}\left[1 + \frac{\cos(2k_x[x - x']) + \cos(2k_y[y - y'])}{2} + \frac{\cos(2k_x[x - x'])\cos(2k_y[y - y'])}{4}\right] d\theta. \tag{3.8}$$

The 2 next integral identities,

$$\int_0^{2\pi}\cos(A\cos\theta)d\theta = \int_0^{2\pi}\cos(A\sin\theta)d\theta = 2\pi J_0(A) \tag{3.9}$$

and

$$\int_0^{2\pi} \cos(A\cos\theta)\cos(A\sin\theta)d\theta = 2\pi J_0(\sqrt{A^2+B^2}), \tag{3.10}$$

yield an analytical expression in terms of 0-th order first kind Bessel functions

$$\langle \phi^2(x,y)\phi^2(x',y')\rangle \propto \frac{1}{A^2}\left[1+\frac{J_0(2k\,|\delta x|)+J_0(2k\,|\delta y|)}{2}+\frac{J_0(2k\delta r)}{4}\right], \tag{3.11}$$

where $\delta x = x' - x$, $\delta y = y' - y$ and $\delta r = r' - r$. Using the same procedure, it can be easily deduced that

$$\langle \phi^2(x,y)\rangle = \frac{1}{A} \tag{3.12}$$

So, finally we obtain the expression of the spatial correlation of the squared eigen modes as

$$\langle \phi^2(x,y)\phi^2(x',y')\rangle = \langle \phi^2\rangle^2\left[1+\frac{J_0(2k\,|\delta x|)+J_0(2k\,|\delta y|)}{2}+\frac{J_0(2k\delta r)}{4}\right]. \tag{3.13}$$

When $x = x'$ and $y = y'$, we find the already known relationship between the fourth order moment and the second order moment of the eigenmodes in a rectangular plate ([2], P.101)

$$\langle \phi^4\rangle = \langle \phi^2\rangle^2\left(\frac{3}{2}\right)^2. \tag{3.14}$$

From Eq. (3.13), we easily deduce that in case of a rectangular plate,

$$F(\delta x,\delta y) = \frac{J_0(2k\,|\delta x|)+J_0(2k\,|\delta y|)}{2}+\frac{J_0(2k\delta r)}{4}. \tag{3.15}$$

## IV. HORIZONTAL COORDINATES OF THE TRANSDUCERS ON THE PLATE

In this section, the coordinates of the transducers are displayed. The origin is the left lower corner of the plate on the same side where the transducers are attached.

TABLE I. Coordinates of the transducers

| Transducer | x(cm) | y(cm) |
|---|---|---|
| 1 | 20.5 | 39 |
| 2 | 17.5 | 25.5 |
| 3 | 30.5 | 34.5 |
| 4 | 29 | 23 |
| 5 | 23 | 18 |


[1] MW Bonilha and FJ Fahy. On the vibration field correlation of randomly excited flat plate structures, i: Theory. *Journal of sound and vibration*, 214(3):443–467, 1998.

[2] Richard H. Lyon and Richard G. DeJong. *Theory and Application of Statistical Energy Analysis*, chapter 4, pages 81–107. Newnes, Boston, second edition edition, 1995.
